# Supplementary material for: Improved Bounds on the Epidemic Threshold of Exact SIS Models on Complex Networks
Source: arXiv:1603.05095 source file (2016-03-16)
Supplement: Supplementary file 1 [file appendix.tex]

%%%%%%%%%%%%%%%%%%%%%%%%%%%%%%%%%%%%%%%%%%%%%%%%%%%%%%%%%%%%%%%%%%%%%%%%%%%%%%%%
\newpage
%%%%%%%%%%%%%%%%%%%%%%%%%%%%%%%%%%%%%%%%%%%%%%%%%%%%%%%%%%%%%%%%%%%%%%%%%%%%%%%%
\appendix
%%%%%%%%%%%%%%%%%%%%%%%%%%%%%%%%%%%%%%%%%%%%%%%%%%%%%%%%%%%%%%%%%%%%%%%%%%%%%%%%
\begin{lemma}
Let G=(V,E) be a star graph on $n$ vertices. If $1-\delta-\beta\geq 0$ and $\delta(1+\delta)<1$, then, for large enough $n$, $\rho(M'')<\rho(M)$.
\end{lemma}
\begin{proof}
First, since $M$ is symmetric and nonnegative, $$\rho(M)=\lambda_{\text{max}}(M) = 1-\delta + \beta \lambda_{max}(A) = 1-\delta + \beta \sqrt{n-1},$$ where we have also used the well-known fact that $\lambda_{max}(A)=\sqrt{n-1}$.

Next, we show that $\rho(M'')<1-\delta + \beta \sqrt{n-1}$. Without loss of generality, assume node $1$ to be the center node of the network. Also, in \eqref{eq:qij_bound}, let $p(t) = (p_1(t),\ldots, p_n(t))^T$, $q_{\text{out}}(t) = (q_{12}(t),\ldots,q_{1n}(t))^T$, $q_{\text{in}}(t) = (q_{21}(t),\ldots,q_{n1}(t))^T$, and $q_E(t) = ( q_{\text{out}}^T(t) ,q^T_{\text{in}}(t) )^T$. With these, the matrix $M''$ takes the form
$$
\begin{bmatrix} (1-\delta) I_n 	&	\beta \Gamma	& \beta\Delta \\
\delta(1-\delta) \Delta^T		&	(1-\delta)(1-\delta-\beta)I_{n-1}		&	\beta\delta I_{n-1}\\
\delta(1-\delta) \Gamma^T	& 	\beta(1+\delta) J_{n-1} - \beta I_{n-1} 	& 	(1-\delta)(1-\delta-\beta)I_{n-1}
\end{bmatrix} ,
$$
where $J_n = 1_n1_n^T$, $\Gamma=\begin{bmatrix} 1_n^T  \\ 0_{(n-1)\times (n-1)}\end{bmatrix}$ and $\Delta=\begin{bmatrix} 0_n^T  \\ I_{(n-1)}\end{bmatrix}$. Note that $M''\geq 0$. 

Define a vector $x = \begin{bmatrix} 1 & \epsilon 1_{n-1}^T & \frac{\alpha}{\sqrt{n-1}}1_{n-1}^T & c1_{n-1}^T  \end{bmatrix}^T$, where $\epsilon, c>0$ and $0<\alpha<1$ are to be determined later. A standard upper bound on the spectral radius of a nonnegative matrix (e.g. \cite[Thm.~8.1.26]{horn2012matrix}) gives
$$
\rho(M'') \leq \max_{1\leq i\leq 3n-2} \rho_i:= \frac{1}{x_i}\sum_{j=1}^{3n-2}M''_{ij}x_j.
$$
It only take some algebra to show that
\begin{align}
\rho_i = \begin{cases}
 1-\delta + \alpha\beta\sqrt{n-1}, & i=1,\\
1-\delta + \beta c/\epsilon, & i=2,\ldots,n,\\
 (1-\delta)(1-\delta-\beta)\alpha \\ ~~~ +(\epsilon\delta(1-\delta) +  \beta\delta c)\sqrt{n-1}, & i=n+1,\ldots,2n-1,\\
 (1-\delta)(1+\delta/c-\delta-\beta) -\frac{\alpha\beta}{c\sqrt{n-1}}\\~~~+ (\alpha/c)\beta(1+\delta)\sqrt{n-1}, & i=2n,\ldots,3n-2.\\
\end{cases}
\end{align}
Now, take $\delta<\alpha<1$, $\max\{\alpha(1+\delta),1\}<c<\frac{\alpha}{\delta}$ (always possible since $\delta(\delta+1)<1$ by assumption) and $0<\epsilon<\frac{\beta(\alpha-\delta c)}{\delta(1-\delta)}$.

\end{proof}

%%%%%%%%%%%%%%%%%%%%%%%%%%%%%%%%%%%%%%%%%%%%%%%%%%%%%%%%%%%%%%%%%%%%%%%%%%%%%%%%
\newpage
...

Now for any $t< t_{mix}(\epsilon)$ we have
\begin{align}
\epsilon &<\mathbb{P}\left( \substack{\text{some nodes are infected at time $t$} \mid \\\text{all nodes were infected at time $0$}} \right)\\
 &\leq \sum\limits_{i=1}^n \mathbb{P}\left( \substack{\text{node $i$ is infected at time $t$} \mid\qquad \\\text{all nodes were infected at time $0$}} \right)\\
 &= 1_{n}^T p(t)\qquad \text{given that $p(0)=1_n$} ,
\end{align}
where we have used the union bound.

Back to the upper-bound on marginals (Eq. \ref{eq:pi_bound}), we have $1_n^Tp(t)\leq 1_n^TMp(t-1)$. Suppose $M$ (e.g. a sufficient condition is to have nonnegative entries) is such that we can ``propagate'' the bound and write
\begin{equation}
1_n^Tp(t)\leq 1_n^TMp(t-1)\leq 1_n^T M^2p(t-2)\leq\dots\leq 1_n^T M^tp(0)
\end{equation}

As a result, for any $t< t_{mix}(\epsilon)$
\begin{equation}\label{eq:bounded}
\epsilon<1_n^TM^t1_n.
\end{equation}

{\bf We want to argue the following
\begin{center}
 If $\rho(M)<1$ then $t_{mix}(\epsilon)\leq O(\log n)$
\end{center}
}
where $\rho(M)$ is the spectral radius of $M$.

{\color{red}If $M$ were symmetric} then \eqref{eq:bounded} implies $\epsilon<n \rho(M)$
(since $M$ is  symmetric, $\rho(M)=\lambda_{max}(M)$).
When $\rho(M)<1$, it follows that $t< \frac{\log \frac{n}{\epsilon}}{-\log \rho(M)}$ for all $t< t_{mix}(\epsilon)$. This concludes the well-known result that when $\beta/\delta<1/\lambda_{\max}(A)$ then $t_{mix}(\epsilon)\leq \frac{\log \frac{n}{\epsilon}}{-\log \rho(M)}=O(\log n)$.

{\color{red}Suppose now that $M$ is {\bf{not} symmetric}}. It would suffice to prove the following, but need some help in the last part...

\begin{lemma}
Let $M\in\mathbb{R}^{n\times n}$. If $\rho(M)<1$, then, there exists $0<\eta<1$ such that  $1^TM^t1\leq \eta^tO(\mathrm{poly}(n)) $ for all $t\geq 0$.
\end{lemma}
\begin{proof}
Since $\rho(M)<1$, by  Lyapunov stability theorem, there exists a unique positive definite matrix $P\succ0$ such that $M^TPM-P\prec0$. Letting $P^{1/2}$ denote the unique square root of $P$ and $N:=P^{1/2}MP^{-1/2}$, it follows easily that 
$ N^TN \prec I_d $, or equivalently $\eta:=\|N\|_2<1$. (Here, $\|N\|_2$ denotes the spectral norm of $N$.) Next, define $y:=P^{1/2}1$ and $x:=P^{-1/2}1$ and note that $1^TM^t1=x^TN^ty$. Thus,
\begin{align}
1^TM^t1=x^TN^ty\leq \|x\|_2\eta^t\|y\|_2 \leq n\eta^T \|P^{1/2}\|_2\|P^{-1/2}\|_2.
\end{align}
{\bf
So, it remains to argue that $ \|P^{1/2}\|_2\|P^{-1/2}\|_2=O(\mathrm{poly}(n))$} {\color{red}???}
\end{proof}

If Lemma is true, then similar to the symmetric case
$$
t< \frac{\log \frac{\mathrm{poly}(n)}{\epsilon}}{-\log \eta} 
$$
for all $t<t_{\text{mix}}(\epsilon)$...
